# Supplementary material for: The shapes of an epidemic: using Functional Data Analysis to characterize COVID-19 in Italy
Source: arXiv:2008.04700 source file (2020-08-11)

## Adjusted p-value heatmap

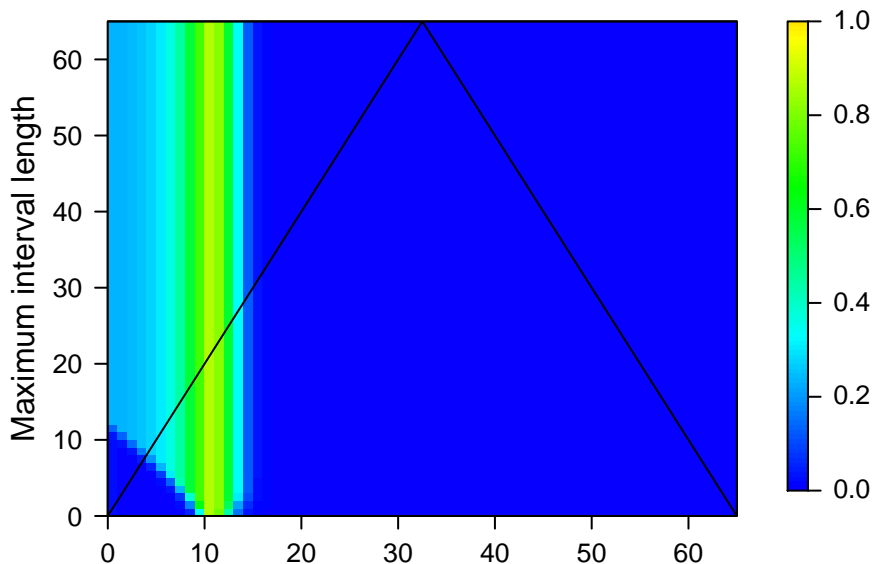

## Adjusted p-values – 65-day scale

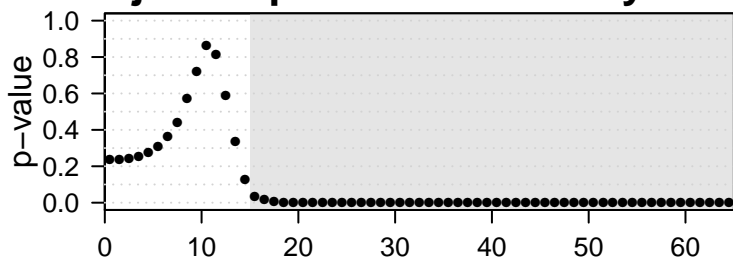

## IWTomics results

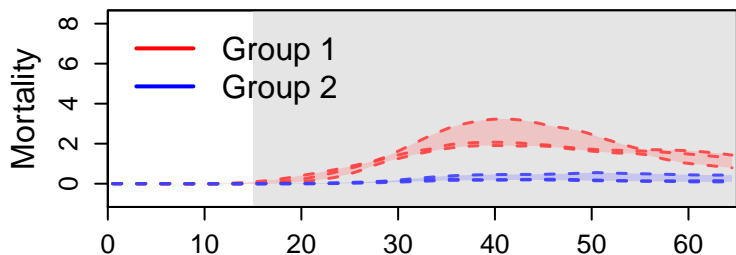

## Adjusted p-value heatmap

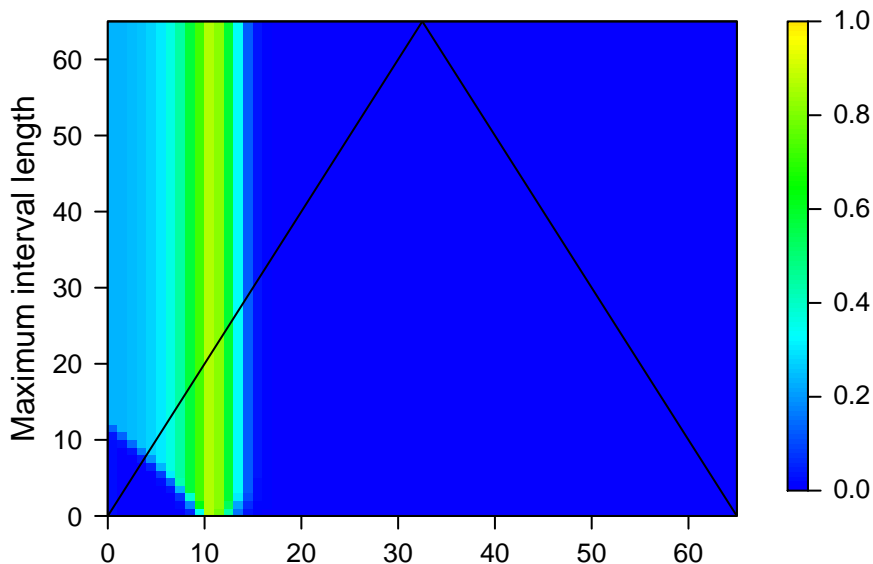

## Adjusted p-values – 65-day scale

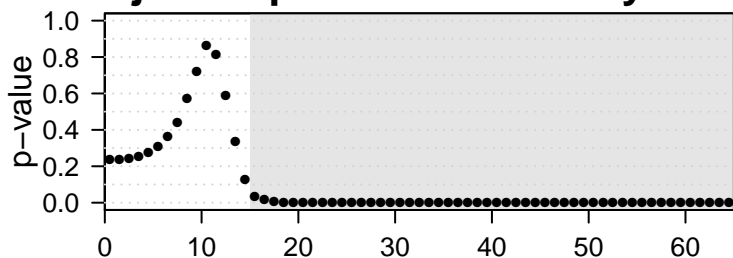

## IWTomics results

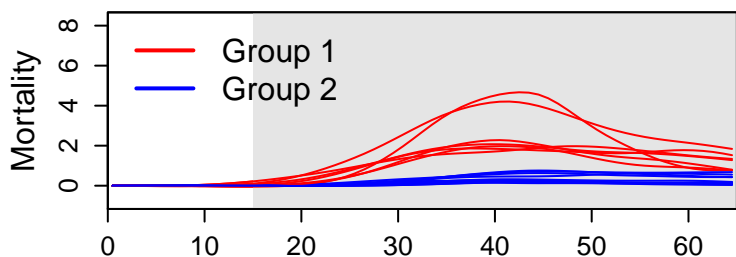

Supplement: Supplementary file 1 [file regions_dpc_IWTomics.pdf]
