# Supplementary material for: The shapes of an epidemic: using Functional Data Analysis to characterize COVID-19 in Italy
Source: arXiv:2008.04700 source file (2020-08-11)

# DPC – Before shifts

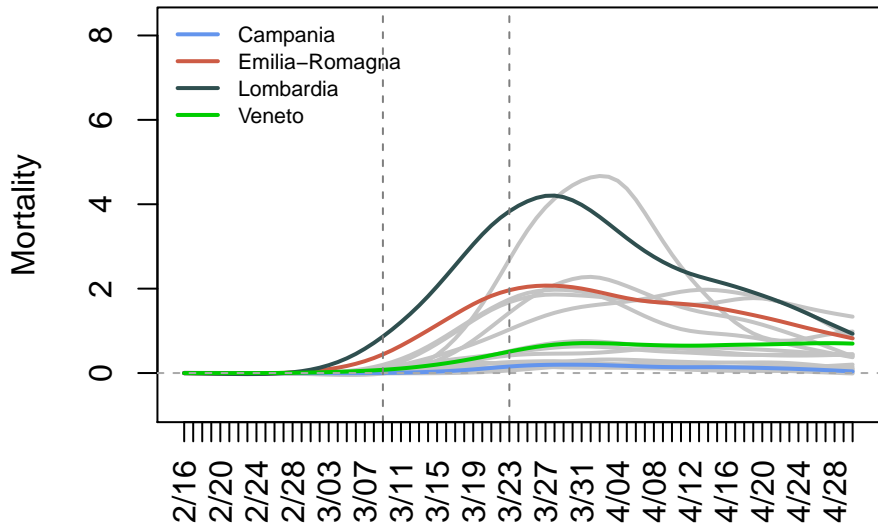

# DPC – After shifts

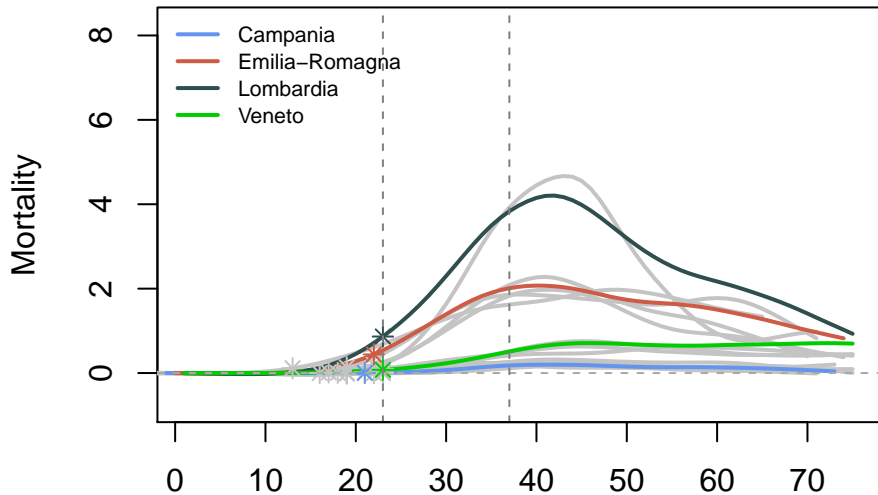

Supplement: Supplementary file 4 [file regions_dpc_smooth_all.pdf]
