# Supplementary material for: The shapes of an epidemic: using Functional Data Analysis to characterize COVID-19 in Italy
Source: arXiv:2008.04700 source file (2020-08-11)

# ProbKMA K=2

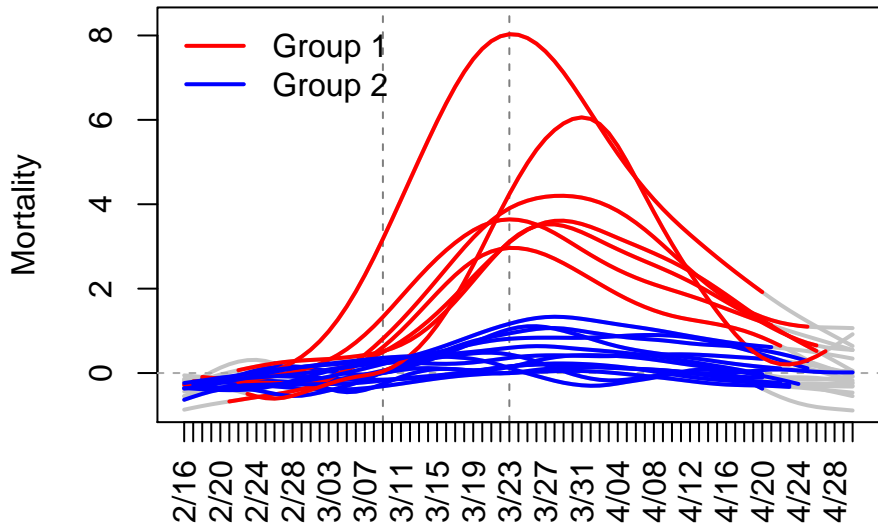

# Group 1

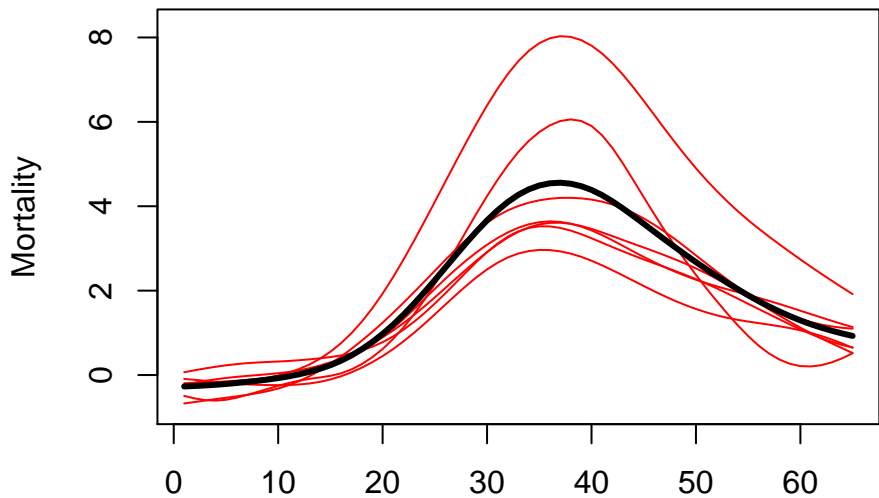

## Group 2

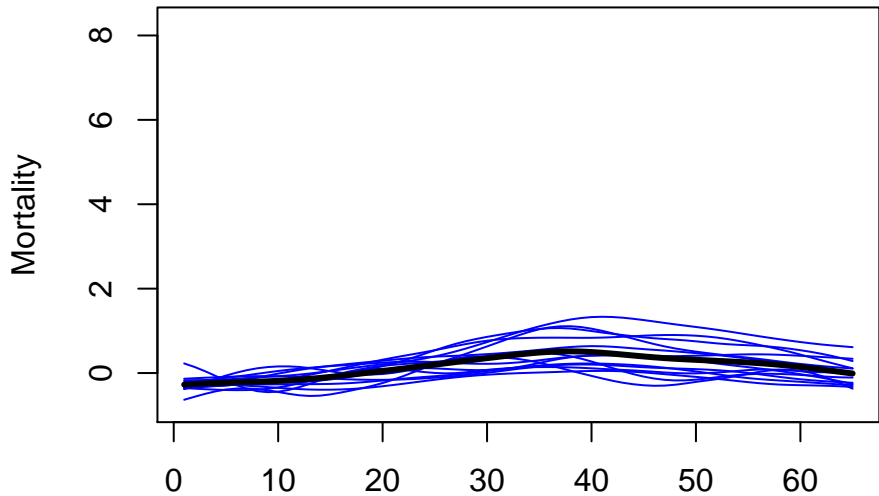

# Shifts

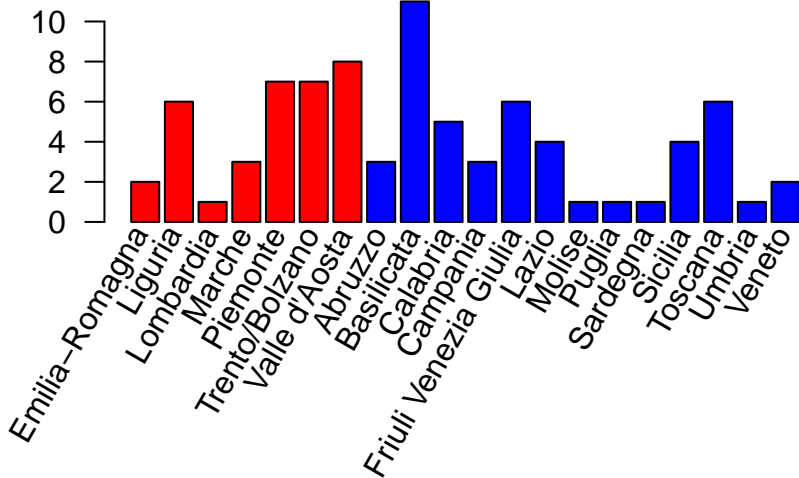

Supplement: Supplementary file 6 [file regions_istat_probKMA_d0_K2.pdf]
