# Supplementary material for: The shapes of an epidemic: using Functional Data Analysis to characterize COVID-19 in Italy
Source: arXiv:2008.04700 source file (2020-08-11)

# ISTAT – Before shifts

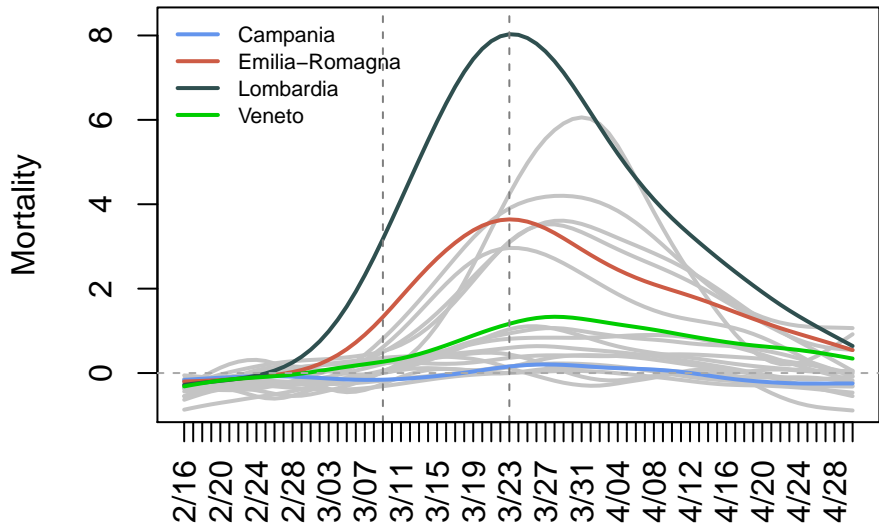

# ISTAT – After shifts

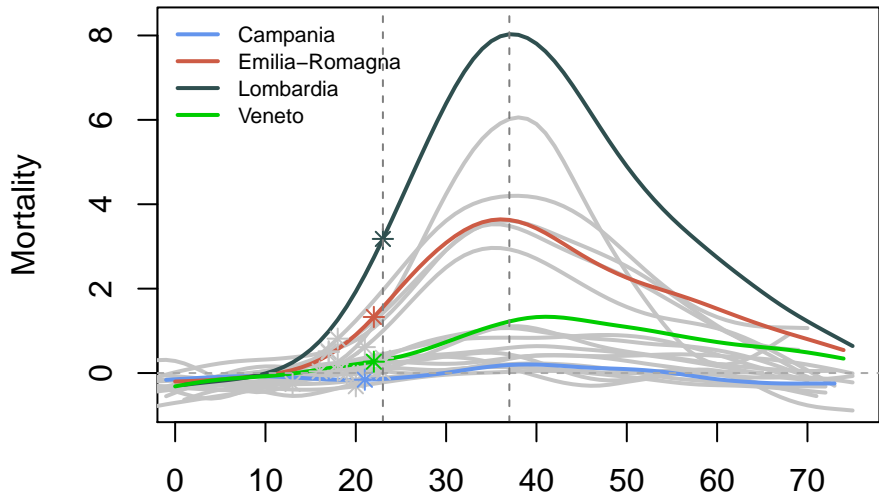

Supplement: Supplementary file 8 [file regions_istat_smooth_all.pdf]
