# Supplementary material for: The shapes of an epidemic: using Functional Data Analysis to characterize COVID-19 in Italy
Source: arXiv:2008.04700 source file (2020-08-11)

# ProbKMA K=3

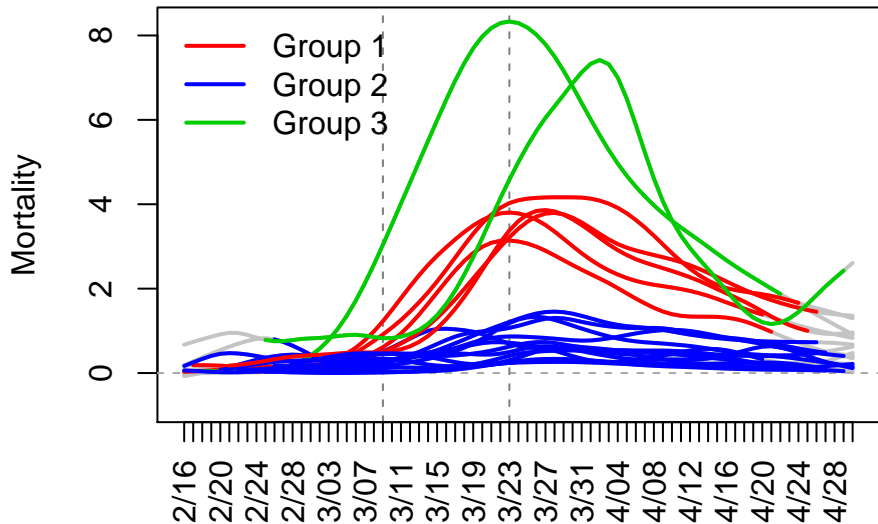

# Group 1

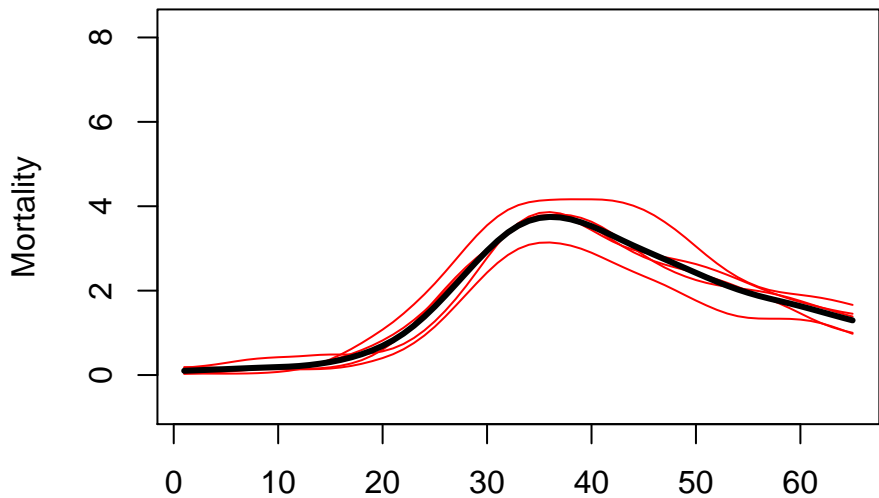

## Group 2

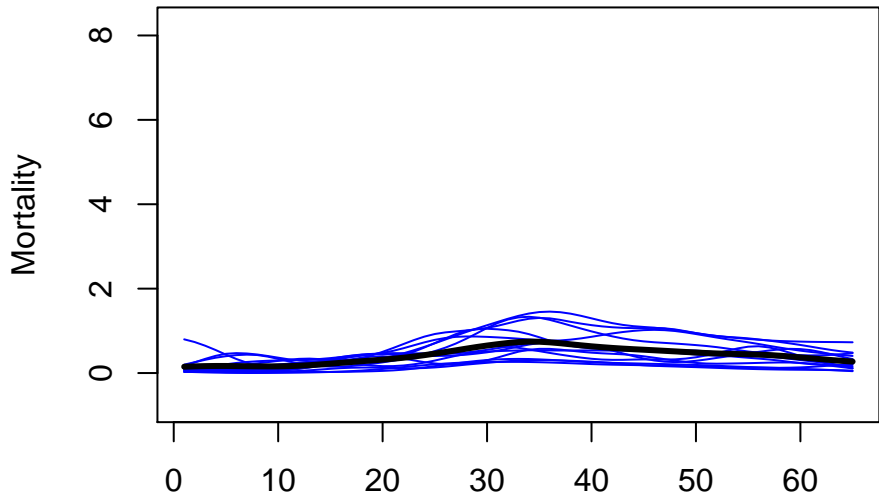

## Group 3

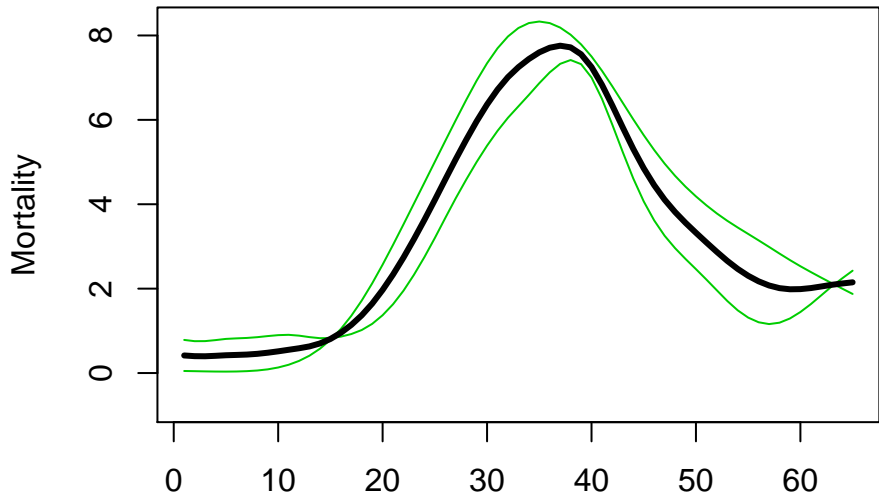

# Shifts

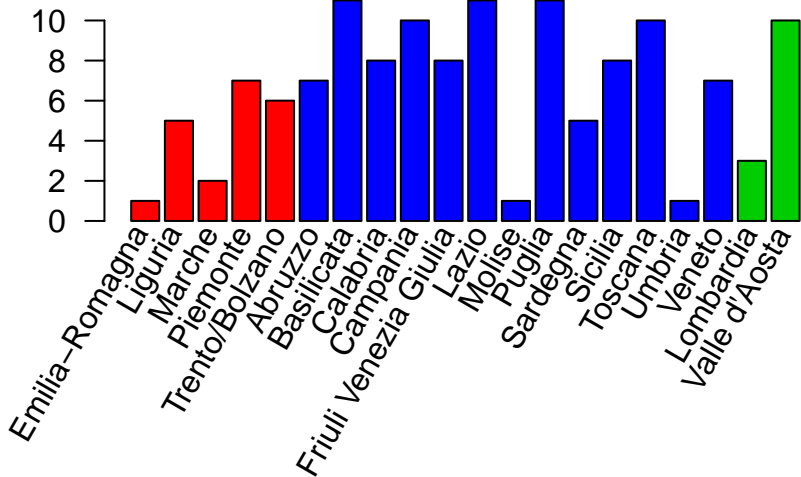

Supplement: Supplementary file 9 [file regions_max_probKMA_d0_K3.pdf]
